# Supplementary material for: The Minimum Leidenfrost Temperature on Smooth Surfaces
Source: arXiv:2010.10480 source file (2021-08-04)
Supplement: Supplementary file 1 [file Supplemental.pdf]

# Supplemental Information – The Minimum Leidenfrost Temperature on Smooth Surfaces

Dana Harvey, Joshua Méndez Harper, and Justin C. Burton*
*Department of Physics, Emory University, Atlanta, Georgia 30322, USA*

## I. SUPPLEMENTARY VIDEOS

**Video S1**: A machined aluminum block with a concave, spherical surface was heated with an embedded ceramic heater, and the temperature was measured with a thermocouple. 2 mm drops of pure DI water were placed onto the surface with a syringe until the drops did not break up or fizzle upon contact. A stable drop formed at $T_+ = 190 \pm 20$°C. The aluminum was then allowed to cool. The drop evaporated and remained levitated until the block temperature fell below boiling (100°C). The video is sped up by a factor of 30.

**Video S2**: A droplet on the same aluminum block as Video S1. The playback has been sped up by a factor of 5. We heated the block well above $T_+$, placed a large droplet on the surface, and the block was cooled rapidly with an air stream until the vapor layer failed. This was a typical experiment for the data represented in Fig. 1b. In this case, the vapor layer failed at $T_- \approx 142$°C, where the radius was $\approx 7.4$ mm.

**Video S3**: The rounded tip of a nickel-plated copper rod was immersed in a bath of DI water at 75°C. The metal was heated using an embedded ceramic heater with an internal thermocouple. When the metal reached $T_+ = 240 \pm 30$°C a stable vapor layer formed. Upon cooling, the vapor layer existed until the metal reached $T_- = 140 \pm 10$°C.

**Video S4**: High-speed video showing the collapse of a vapor layer at a surface temperature $T_s = T_-$. The original video was recorded at 33,000 fps, and the playback rate is 1,650 times slower then real time. A single failure point resulted in a wetting front that traveled at the capillary velocity ($\gamma/\eta_{\rm w} \approx 210$ m/s), followed by nucleate boiling.

## II. EXPERIMENTAL APPARATUS

Our experimental Leidenfrost system was designed for high-speed measurements of the dynamics of the vapor layer. The apparatus consisted of metal rods with hemispherical tips immersed in a bath of water with an adjustable salt concentration (Fig. 2a in the main text). We controlled the immersion depth of the rod, $H$, the temperature of the bath, $T_l$, the temperature of the rod, $T_s$, and the position of the rod in the bath. $H$ and $T_l$ were controlled using an exterior water bath. The exterior water bath rested on a hot plate so that $T_l \approx 75$°C. The bath was connected by a small tube to the experiment so that water could be gravitationally siphoned in order to keep $H$ constant. We also used silicon heaters glued to the experimental chamber to keep the water temperature consistent. $T_l$ was measured using a k-type thermocouple immersed in the bath.

The upper metal electrodes used in the experiment were cylinders of length 8.90 cm and radii 7.94 mm. They were constructed from titanium alloy, brass, and copper. The brass and copper were electroplated with nickel to resist corrosion. At one end there was a hemispherical tip with radius 7.94 mm, and at the other end was a lip of radius 1.11 cm. The lip held the electrode in place and housed electrical connections to the BNC cables. The lip rested on ceramic, insulating washers attached to a vertical, linear motion system allowing us to raise and lower the heated electrode. The lower electrode, same geometry, but 6.35 cm long, was fully immersed in the bath and machined from titanium alloy so that it was resistant to salt water (Fig. 2a in the main text). The electrodes were heated using a cylindrical ceramic heater that was cemented in the center of the rod. A K-type thermocouple at the end of the ceramic heater measured $T_s$ near the tip.

Fig. S1 shows a schematic of the measurement system, including the RG58C/U cables, which are important for correctly interpreting the electrical impedance of the Leidenfrost system. $Z_{\rm unknown}$ represents the complex impedance of the Leidenfrost system (Fig. 2b in the main text), including any parasitic capacitance or inductance. During measurements, a sinusoidal carrier signal with frequency $f = 10$ MHz and variable amplitude = 0.2-3.5 V was generated by an Agilent 33220A function generator. The signal was split into two cables of identical length ($S1$), and passed through both $Z_{\rm unknown}$ and a 6 dB pi-pad attenuator before being acquired by two channels of a National Instruments PCI-5153 computer-based oscilloscope. The attenuator minimized noise in the final measurement by forcing the voltage range of each channel to be the same [1]. Since the impedance of both channels and the attenuator was 50 Ω, only reflections above $Z_{\rm unknown}$ were considered in the model.

While we used the same carrier wave frequency for all experiments, we sampled the data differently. For short time scales, we used a sample rate of 200 MS/s for 50 ms of data, for a total of 10 MS (here "MS" refers to

* justin.c.burton@emory.edu

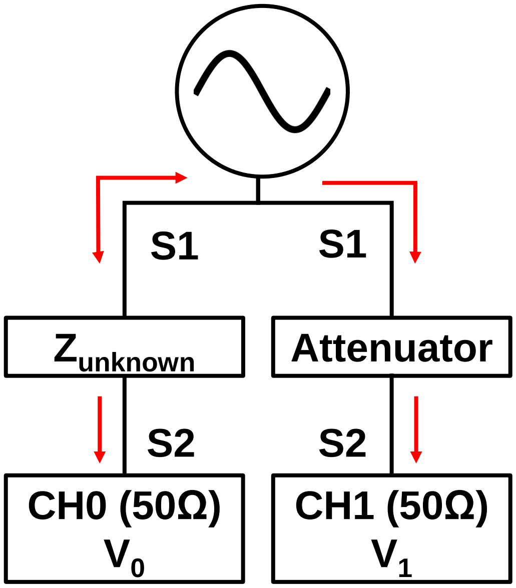


FIG. S1. Measurement system used to determine $Z_{\text{unknown}}$ of the Leidenfrost system. The carrier wave (10 MHz) traveled along RG58C/U cables of lengths $S1$ and $S2$. The telegraphers equations are solved along each length of cable. Arrows indicate allowed directions of current along each cable. By simultaneously measuring $V_0$ and $V_1$, we could determine $Z_{\text{unknown}}$.

"Megasamples"). This is equivalent to 20 sampled points per cycle for the 10 MHz carrier wave. We wrote a custom LabVIEW program that acts as a lock-in amplifier to extract the 10 MHz amplitude for each cycle, resulting in a total of 500,000 data points for the data shown in Fig. 3 (main text). For some experiments, such as those shown in Figs. 2 and 4 in the main text, the thickness, $d$, is measured over many minutes. For these measurements, we averaged 800 samples at 100 MS/s to calculate the thickness of the vapor layer in 1 s intervals. Additionally, $T_s$ and $T_l$ were also measured every second.

## III. ELECTRICAL MEASUREMENTS OF THE VAPOR LAYER

In order to measure $Z_{\text{unknown}}$, and ultimately the thickness of the vapor layer, we solved the telegraphers equations on each cable, and matched the boundary conditions at $Z_{\text{unknown}}$ and the attenuator (Fig S1). We ignored losses and assumed a capacitance, $C_c$, and inductance, $L_c$, per unit length of cable. Along the length $x$ of each cable, the voltage $V$ and current $I$ are determined by:

$$\frac{dV}{dx} = -L_c \frac{dI}{dt}, \tag{1}$$
$$\frac{dI}{dx} = -C_c \frac{dV}{dt}. \tag{2}$$

Assuming a plane wave ansatz, $V = V_c e^{i(k_c x - \omega t)}$ and $I = V/\sqrt{L_c/C_c}$, where $V_c$ is the amplitude, $k_c$ is the wave vector, and $\omega = 2\pi f$ is the angular frequency, we solve for the real and imaginary components of $Z_{\text{unknown}}$, $Z_R$ and $Z_I$, respectively.

By taking the real part of the signals, the resulting expressions for $Z_R$ and $Z_I$ can be written in terms of the measured signals (CH0 and CH1, Fig. S1). For each channel, the voltage can be written as a sum of sine and cosine:

$$V_0 = A_0 \cos \omega t + B_0 \sin \omega t \tag{3}$$
$$V_1 = A_1 \cos \omega t + B_1 \sin \omega t. \tag{4}$$

A custom LabVIEW program extracts $A_0$, $A_1$, $B_0$, and $B_1$ for each cycle of oscillation of the 10 MHz carrier wave. Thus, the amplitudes are sampled every 100 ns. $Z_R$ and $Z_I$ are then computed using the following relations:

$$Z_R = \frac{-R_{in}}{A_0^2 + B_0^2} \Bigg( A_0^2 - A_0 A_1 A_F + B_0 (B_0 - A_F B_1) + A_F (A_1 B_0 - A_0 B_1) \tan\left(\frac{S\omega}{v}\right) \Bigg), \tag{5}$$

$$Z_I = \frac{R_{in}}{A_0^2 + B_0^2} \Bigg( - A_1 A_F B_0 + A_0 A_F B_1 + (A_0^2 - A_0 A_1 A_F + B_0 (B_0 - A_F B_1)) \tan\left(\frac{S\omega}{v}\right) \Bigg). \tag{6}$$

where $R_{\text{in}} = 50\ \Omega$ is the input impedance of the oscilloscope channels, $S = S1 = 1.1$ m, $v = 0.65c$ is the wave speed on the cable (relative to the speed of light $c$), and $A_F = 2.02$ is the measured voltage attenuation ratio for the 6 dB attenuator.

Ultimately we want to relate $Z_R$ and $Z_I$ to $R_0$, $C_v$, and $C_\lambda$, as shown in Fig. 2b in the main text. Since $C_v$ and $C_\lambda$ are summed in parallel, we can only measure the total capacitance $C_v + C_\lambda$. Thus, $R_0$ and $C_v + C_\lambda$ can be written as:

$$R_0 = Z_R, \tag{7}$$
$$C_v + C_\lambda = \frac{1}{\omega (Z_I + L_0 \omega)}. \tag{8}$$

While $C_v + C_\lambda$ and $R_0$ are functions of time, we assume the parasitic inductance $L_0$ is constant. In order to measure $L_0$ in the experiments, we use the fact that the impedance associated with $C_\lambda$ is almost negligible when there is a fully-formed double layer. The length scale associated with charge separation is $\lambda \approx 1 - 10$ nm [2], which is more than 3 orders of magnitude smaller than the typical vapor layer thickness $d$ (Fig. S2). Prior to collapse, there is no liquid-solid contact so $C_\lambda = 0$. Well after collapse, when there is significant liquid-solid contact, $C_v = 0$ and $C_\lambda < 3\ \mu$F for the centimeter-scale electrodes in our experiment [2]. At $f = \omega/2\pi = 10$ MHz, the corresponding impedance is $1/|\omega C_\lambda| < 0.045$

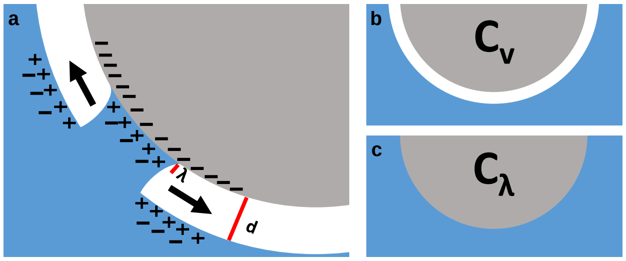


FIG. S2. (a) During the collapse of a vapor layer with thickness $d$, the capacitance rapidly changes due to the formation of a double layer of thickness $\lambda \ll d$. (b) Prior to collapse, the capacitance is solely determined by the capacitance of the vapor layer, $C_v$. (c) After collapse, it is the double layer capacitance, $C_\lambda$, which dominates the parallel combination.

$\Omega$. Thus, we can ignore the impedance due to $C_\lambda$ and assume $L_0 = Z_I/\omega$ when there is a double layer. For our experiments, $L_0 \lesssim 1$ $\mu$H. We then use this measured value of $L_0$ for each experiment and apply it to data before, during, and after the collapse.

The vapor layer collapses by the propagation of a wetting front at $\approx 25$ ms, followed by an explosion of bubbles (Video S4). A schematic of the touchdown and propagating wave is shown in Fig. S2a. Prior to collapse, the resistance is mostly due to the bulk ions in the water, and there is no liquid-solid contact, so $C_\lambda = 0$ (Fig. S2b). The transition from a vapor layer capacitor to a Debye layer capacitor can be thought of as liquid bridges contacting the hot surface, Fig. S2a. We assume that the transition is so fast that $d$ remains constant as the wetting front grows. As the surface area of the liquid bridges grows, $C_\lambda$ will grow rapidly and overtake the capacitance. Since $\lambda$ is orders of magnitude smaller then $d$, the surface area of contact can still be small when $C_v$ becomes negligible. At this point the capacitance measurement becomes unreliable.

## IV. COMPUTING THE VAPOR LAYER THICKNESS

As derived in the main text of the paper, the thickness of the vapor layer, $d$, is calculated from a geometric model combining a concentric hemispherical capacitor with a sphere-plane capacitor. The resulting relationship between $C_v$ and $d$ is

$$\frac{C_v - C_0}{2\pi R\epsilon_v} = \frac{cH}{d} + \ln\left(\frac{R}{d}\right), \tag{9}$$

where $R = 7.9$mm is the radius of curvature of the tip of the rod, $C_v$ is the capacitance when a vapor layer is present (Fig. S2b), $c = 0.58$ is a numerical correction to the simple model accounting for the curved water surface, $H$ is the immersion depth as measured from the tip of the electrode to the water surface far from the interface (Fig. 2c), $C_0 = 1.85$ pF is a constant offset to the capacitance, and $\epsilon_v = 1.0057\epsilon_0$ is the dielectric constant for water vapor.

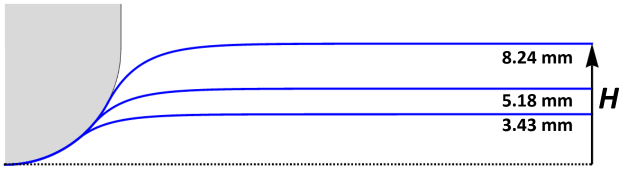


FIG. S3. Piecewise water surface profiles for a 30 $\mu$m vapor layer at various values of $H$. When computing capacitance in the COMSOL model, these profiles are rotated about the z axis.

In order to verify this approximation and compute the constants $c$ and $C_0$, we modeled our geometry and computed the capacitance in COMSOL [3]. We used a two-dimensional axisymmetric electrostatic simulation with radial coordinate $r$ and axial coordinate $z$. The simulation space was a cylinder of radius $R_{max} = 4$ cm and height 11 cm. The top electrode was a cylinder centered and fixed to the top of the space with radius $R = 7.9$ mm and height 4.5 cm. A hemispherical tip of radius $R$ was added to the top electrode. The full profile of the water surface was made by patching an arc of radius $R + d$ centered on the tip to a surface profile, $f(r)$, given by balancing surface tension and gravitational forces [4]:

$$f'' + \frac{f'}{r} = \frac{g\rho_l}{\gamma} f - P_0. \tag{10}$$

Here, $\rho_l$ is the liquid density, $g$ the acceleration due to gravity, $\gamma$ is the surface tension, and $P_0$ is a constant pressure. The prime denotes differentiation with respect to $r$. We have also assumed that the interface profile is shallow, i.e. $f'(r) << 0$, to simplify the full expression for the curvature and produce a linear equation.

The outer boundary conditions were $f(R_{max}) = H$ and $f'(R_{max}) = 0$. The curved outer surface given by Eq. 10 was patched at a point $r_0$ to the inner circular arc with the requirements of continuity in $f$ and $f'$, which then determined the appropriate values of $r_0$ and $P_0$. The equations are solved analytically using Mathematica, resulting in a complex expression for $f$ containing Bessel functions. We constructed many water surface profiles for different values of $d$ and $H$, and a few examples are shown in Fig. S3. In the electrostatic model the rod is treated as one metal electrode and the water surface is treated as the other with vacuum between them.

Figure 2d in the main text shows the resulting capacitance from the simulation when varying $d$ from 10-100 $\mu$m and $H$ from 1.3 - 8.3mm. In experiments, $H$ varied from 3-8 mm (Fig S5). The dashed line in Fig. 2d is Eq. 9 with $c = 0.58$ and $C_0 = 1.85$ pF. The agreement is very good. Using those values for $c$ and $C_0$ makes Eq. 9 a reliable and quantitative way to solve for $d$ from measurements of $C_v$.

## V. HYSTERESIS EXPERIMENTS

As shown in Fig. 2e in the main text, the temperature at which the vapor layer forms ($T_+$) is much higher than the temperature at which it eventually collapses ($T_-$). To measure this hysteresis, the upper metal electrode was immersed into the bath before heating. The initial temperature of the bath was set at $T_l = 75°$C. We used the nickel plated copper rod and pure DI water. Salt was not added so as to avoid deposition of salt on the surface during the nucleate boiling regime while heating. The upper electrode was then heated until a stable vapor layer formed when $T_s \approx T_+$ (Video S3).

We measured $d$, $T_s$, and $T_l$ every second. For all experiments, we sampled the 10 MHz signal at 100 MS/s and averaged 800 cycles every second to form one data point. After the vapor layer formed, the heater was turned off and the rod was allowed to cool. Eventually, at a lower temperature $T_-$, the vapor layer failed and violent boiling ensued. We found that on average, $T_- = 140 \pm 10°$C and $T_+ = 240 \pm 30°$C.

We observed similar hysteresis in Leidenfrost drops. In these experiments, we used an aluminum substrate with a concave polished surface. The substrate is heated with an embedded ceramic heater. A k-type thermocouple read the temperature of the aluminum near the drop. Water was periodically dropped on the surface until a vapor layer formed instantaneously at $T_+ = 190 \pm 20°$C. The heater was then turned off and the aluminum cooled until the vapor layer under the droplet failed at $T_-$. Some drops could levitate even below the boiling point, $T_- < 100°$C (Video S1).

## VI. COOLING EXPERIMENTS

In order to measure $d$ versus $T_s$, we performed experiments where the upper electrode was heated well above $T_+$, to 500-600°C, before immersing it in the liquid bath. The initial temperature of the bath was set at $T_l = 75°$C. Upon lowering the upper electrode into the bath at a fixed distance from the bottom electrode, a vapor layer instantly formed around the tip with no liquid-solid contact. We used the same sampling rate as in the hysteresis experiments, described above. We measured $d$, $T_s$, $T_l$, and $H$ every second until $T_s = T_-$ at failure. Time series for $T_s$ and $d$ are shown in Fig. S4 for titanium and copper over many experiments and salt concentrations.

We tested 3 metals with varying thermal conductivity, titanium (7 W/m·K), brass (115 W/m·K), and copper (390 W/m·K). Each rod was polished with micron-scale lapping compound, resulting in a reflective finish. The copper and brass rods were electroplated with nickel to inhibit surface corrosion during rapid heating and cooling over many experiments in salt water. For each metal, we used NaCl concentrations from 0-0.6 M, where the upper range roughly corresponds to the concentration of NaCl in sea water. Over many runs it is difficult to see any

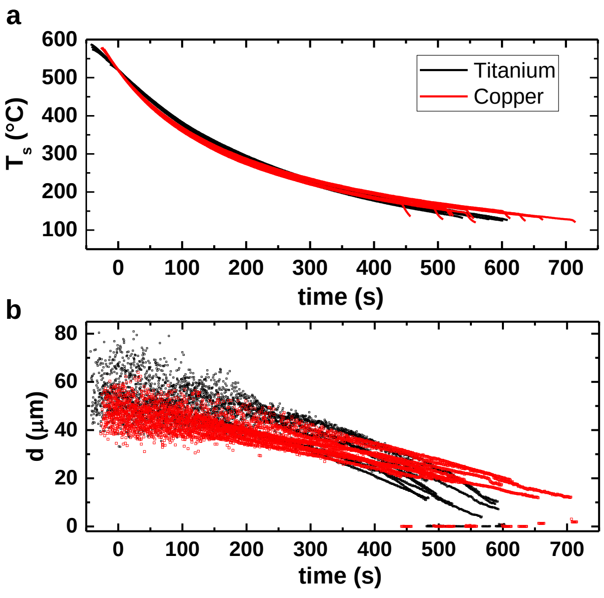


FIG. S4. Series of individual experiments showing the surface temperature $T_s$ versus time for titanium and copper (a), and the thickness $d$ versus time for titanium and copper (b). All data have been shifted in time so that $T_s = 520°$C at the origin. Black (Red) lines and dots are for titanium (copper) experiments. There are slight differences between the two metals in the time series due to their heat capacity. Failure occurred at nearly the same $T_-$ for both metals.

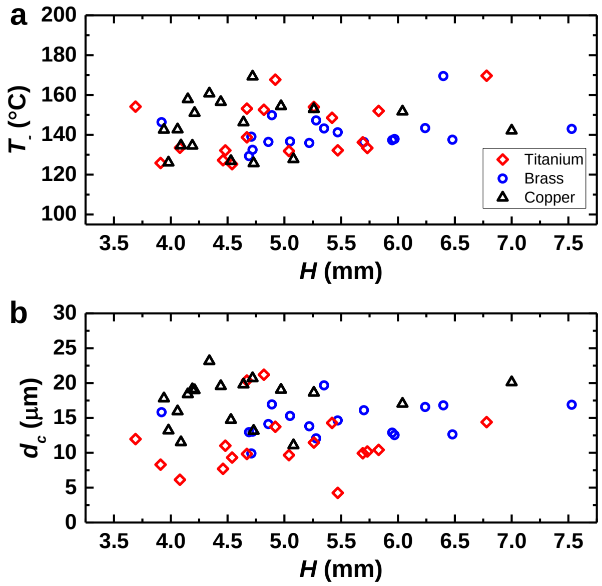


FIG. S5. The failure temperature, $T_-$ (a), and the thickness at failure, $d_c$ (b), as functions of the immersion depth, $H$. Data are shown for 3 materials, as indicated in the legend.

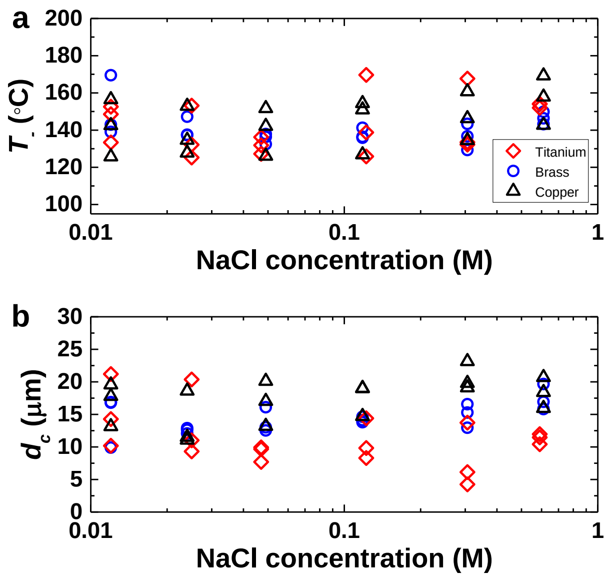


FIG. S6. The failure temperature, $T_-$ (a), and the thickness at failure, $d_c$ (b), as functions of NaCl concentration. Data are shown for 3 materials, as indicated in the legend.

difference in the cooling curves for a given metal when changing the salt concentration. All the data in these graphs have been shifted in time so that $T_s = 520°C$ at the origin. There is slight variation between the cooling curves for the different metals. It took slightly longer for the copper rod to cool under the same conditions as the titanium (Fig. S4a). This is expected since the heat capacity of copper is larger than titanium and most of the cooling is from the ambient environment, not through the vapor layer. The variation between experiments for a given metal did not correlate with salt concentration (e.g. Fig. 4b in the main text and Fig S6). Most importantly, the cooling curves show that on average $T_- = 140 \pm 10°C$ for both metals.

As the metal cooled, $d$ tended to follow the same decay rate between different experiments (Fig. S4b). Noise existed at large $d$ in our experiments because our measurement was not sensitive to changes in vapor layer capacitance for thick layers. However, the decay rates for each metal were distinct since $d$ depended mostly on $T_s$ (Fig. 4a in the main text). Since the copper cooled slower, the corresponding vapor layer thickness also decreased more slowly, although this difference was subtle.

As shown in Fig. 4b in the main text, the failure thickness, $d_c$, and minimum temperature, $T_-$, did not significantly depend on the material properties. Additionally, these values did not depend on the immersion depth, $H$, or on the NaCl concentration. In Fig. S5a, we plot $T_-$ as a function of $H$ at collapse, and in Fig. S5b we plot $d_c$ as a function of $H$ at collapse. Neither $T_-$ nor $d_c$ is strongly affected by $H$. It is important to note that $H$ can directly tell us the surface area of the Leidenfrost vapor layer. Values of $H$ range from 3.7-7.6 mm corresponding to surface areas of 89-210 mm$^2$. The fact that the size does not affect the failure temperature in this regime supports our analogous findings in the drop experiments (Fig. 1b in the main text). In Fig. S6, we plot $T_-$ and $d_c$ as functions of NaCl concentration, where the colors represent the different metals. Again we see that $T_-$ is independent of NaCl concentration. With one standard deviation $T_- = 140 \pm 10°C$ for all concentrations and metals.

For the cooling experiments with Leidenfrost droplets of pure DI water, an aluminium block was heated to well over 200°C and a large drop was deposited on the surface. The system was allowed to cool by means of an air stream blown onto the aluminum block from below. The solid temperature and radius of the drop were recorded in time (Video S2). The failure temperature, $T_-$, decreased sharply at small drop sizes. The results shown in Fig. 1b in the main text give the radius and temperature of many drops at the failure point. In these experiments, $T_-$ was significantly less than $T_+$. We also note that for drop sizes above the capillary length, $l_c$, the minimum failure temperature was $T_- \approx 140°C$. This indicates that it is not the size of the droplet, but the vapor layer thickness that determined $T_-$.

[1] J. D. Paulsen, J. C. Burton, and S. R. Nagel, Viscous to inertial crossover in liquid drop coalescence, PRL **106**, 114501 (2011).
[2] M. Khademi and D. P. J. Barz, Structure of the electrical double layer revisited: Electrode capacitance in aqueous solutions, Langmuir **36**, 4250 (2020).
[3] COMSOL Multiphysics®, v. 5.3. COMSOL AB, Stockholm, Sweden (2020).
[4] J. C. Burtin, F. M. Huisman, P. Alison, D. Rogerson, and P. Taborek, Experimental and numerical investigation of the equilibrium geometry of liquid lenses, Langmuir Article **26**, 15316–15324 (2010).
